# Supplementary material for: Multi-orbital model reveals second-order topological insulator in 1H-transition metal dichalcogenide
Source: arXiv:2108.12855 source file (2021-08-29)
Supplement: Supplementary file 1 [file SupplementalMaterials.pdf]

# Supplemental Materials: Multi-orbital model reveals second-order topological insulator in 1H-transition metal dichalcogenide


Jiang Zeng,[1,*] Haiwen Liu,[2] Hua Jiang,[3] Qing-Feng Sun,[1,4,5] and X. C. Xie[1,4,5,†]

[1] International Center for Quantum Materials, School of Physics, Peking University, Beijing, China
[2] Center for Advanced Quantum Studies, Department of Physics, Beijing Normal University, Beijing 100875, China
[3] School of Physical Science and Technology, Soochow University, Suzhou 215006, China
[4] Beijing Academy of Quantum Information Sciences, Beijing, China
[5] CAS Center for Excellence in Topological Quantum Computation, University of Chinese Academy of Sciences, Beijing, China


## Supplemental A: Electronic band structures of the six 1H-$MX_2$ monolayers

Atomic structures of the six monolayer transition metal dichalcogenides 1H-MX2 were fully relaxed using first-principles density functional theory (DFT) [1]. The calculations were performed by the Vienna Ab initio Simulation Package (VASP) [2, 3] with projector-augmented wave method [4] and exchange-correlation functional in the Perdew-Berke-Ernzerhof's form [5] within the generalized-gradient approximation [6, 7]. We used an energy cutoff of 400 eV and maximum residual force less than 0.001 eV/Å. The Monkhorst-Pack k-point sampling [8] of 8×8×1 was adopted for the Brillouin zone integration, and a large vacuum region of more than 15 Å was applied in order to minimize image interactions from the periodic boundary condition. The DFT results were adopted as inputs to construct the maximally localized Wannier functions, using the WANNIER90 [9] code and the tight-binding method to calculate the Berry connection and topological invariants. The calculated electronic band structures of the six monolayer transition metal dichalcogenides 1H-MX2 are shown in Fig. S1. The hopping parameters are listed in Table SI.

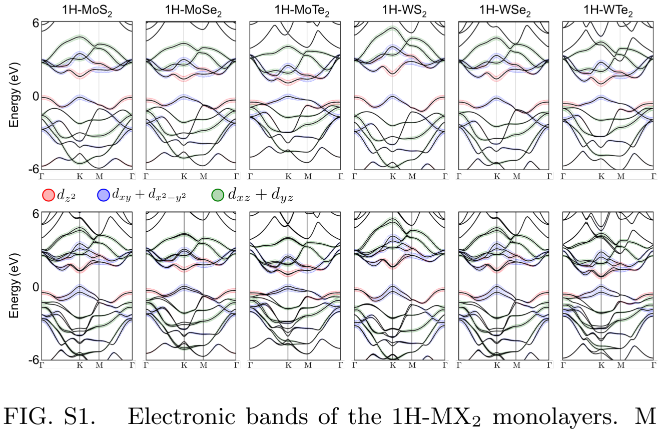


FIG. S1. Electronic bands of the 1H-$MX_2$ monolayers. M stands for (W, Mo) and X stands for (Te, Se, S). The upper (lower) panels are orbital projected bands without (with) considering spin orbital coupling. Colored circles represent contributions from different M-$d$-orbitals. The Fermi energy $E_\mathrm{f}$ is set to be zero as a reference.

## Supplemental B: Symmetry faithful tight-binding Hamiltonian and bulk polarization

Here, we develop a symmetry-based multi-orbital tight-binding model. From early theoretical studies, we know that the Bloch states of 1H-$MX_2$ monolayer near the Fermi level mostly consist of M-$d$-orbitals, especially the $d_{z^2}$, $d_{xy}$, and $d_{x^2-y^2}$ orbitals. In previous work [10], a symmetry-based tight-binding model has been constructed. Here, we redefine the basis as $\psi = \mathbf{R}\tilde{\psi}$, where

$$\psi = \begin{bmatrix} d_1 \\ d_2 \\ d_3 \end{bmatrix}, \ \tilde{\psi} = \begin{bmatrix} \tilde{d}_1 \\ \tilde{d}_2 \\ \tilde{d}_3 \end{bmatrix} = \begin{bmatrix} d_{z}2 \\ d_{xy} \\ d_{x^2-y^2} \end{bmatrix}, \ \mathbf{R} = \begin{bmatrix} \frac{\sqrt{3}}{3} & 0 & \frac{\sqrt{6}}{3} \\ \frac{\sqrt{3}}{3} & -\frac{\sqrt{2}}{2} & -\frac{\sqrt{6}}{6} \\ \frac{\sqrt{3}}{3} & \frac{\sqrt{2}}{2} & -\frac{\sqrt{6}}{6} \end{bmatrix}. \quad (1)$$

Thus, the tight-binding Hamiltonian $H = H_\mathrm{s} + H'$ can be expressed as

$$H_\mathrm{s} = \sum_{\boldsymbol{r};i;j;k} \frac{t_{23} + t_{32} \pm (t_{23} - t_{32})\epsilon_{ijk}}{2} d^\dagger_{\boldsymbol{r},i} d_{\boldsymbol{r}\pm\boldsymbol{a}_k,j} |\epsilon_{ijk}| + t_\mathrm{E} \sum_{\boldsymbol{r};i;j} d^\dagger_{\boldsymbol{r},i} d_{\boldsymbol{r},j}, \quad (2)$$

$$H' = \sum_{\boldsymbol{r};i;j;k} \frac{t_{31} + t_{13} \pm (t_{31} - t_{13})\epsilon_{ijk}}{2} (d^\dagger_{\boldsymbol{r},i} d_{\boldsymbol{r}\pm\boldsymbol{a}_i,j} + d^\dagger_{\boldsymbol{r},j} d_{\boldsymbol{r}\mp\boldsymbol{a}_i,i}) + E_0 \sum_{\boldsymbol{r};i} d^\dagger_{\boldsymbol{r},i} d_{\boldsymbol{r},i} + t_{11} \sum_{\boldsymbol{r};i} d^\dagger_{\boldsymbol{r},i} d_{\boldsymbol{r}\pm\boldsymbol{a}_i,i} + t_{22} \sum_{\boldsymbol{r};i;j} d^\dagger_{\boldsymbol{r},i} d_{\boldsymbol{r}\pm\boldsymbol{a}_j,i} (1 - \delta_{ij}), \quad (3)$$

where $i, j, k = 1 - 3$; $\boldsymbol{r}$ runs all the sites; the $t_{ij}$ ($\tilde{t}_{ij}$) is the hopping between the $d_i(\tilde{d}_i)$ orbital to $d_j(\tilde{d}_j)$ orbital on its nearest neighbor site along $\boldsymbol{a}_1$, $t_\mathrm{E} = \frac{\epsilon_1 - \epsilon_2}{3}$ describes the energy split between the $d_{z^2}$ ($\epsilon_1$), $d_{xy}$ ($\epsilon_2$), and $d_{x^2-y^2}$ ($\epsilon_2$) orbitals due to the crystal field effects, $E_0$ tunes the Fermi energy, $\delta_{ij}$ is the Kronecker delta function, and $\epsilon_{ijk}$ is the Levi-Civita Symbol. Figure S2 shows the schematic lattice diagrams. Please also refer to Ref. [11] for similar Hamiltonian. It notes that the basis $\tilde{\psi}$ rather than $\psi$ is usually used, when one use first-principles based WANNIER90 software to construct the tight-binding Hamiltonian. The hopping parameters follow the relation: $\boldsymbol{t} = \mathbf{R}\tilde{\boldsymbol{t}}\mathbf{R}^\mathrm{T}$. The first-principle calculated parameters are listed in Table SI.

The $D_{3h}$ symmetry is directly manifested in each term, which allows us to consider each term independently. For a TMD monolayer, we considered three $d$-orbitals on each site and there are 6 nearest-neighbor sites. For each site,

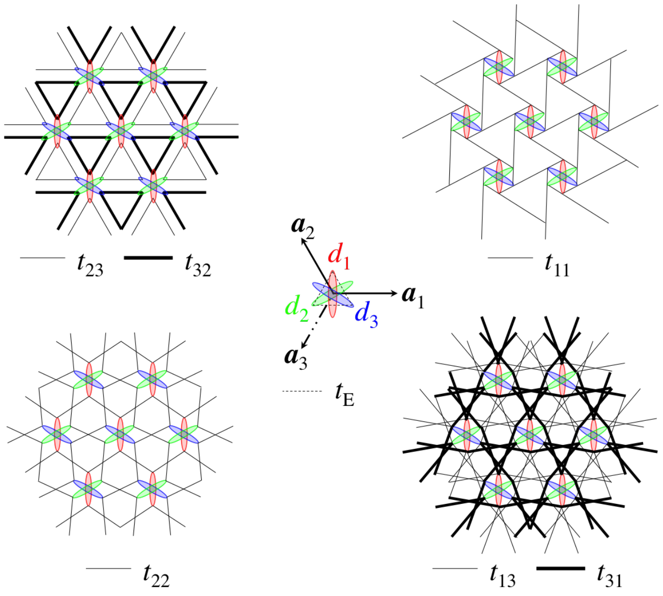


FIG. S2. Schematic lattice diagrams of the tight-binding Hamiltonian $H = H_{\rm s} + H'$ expressed in Eqs. (S2) and (S3). For convenience, a third lattice vector is defined as $\boldsymbol{a}_3 = -\boldsymbol{a}_1 - \boldsymbol{a}_2$ to simplify the expression in Eqs. (S2) and (S3).

TABLE S1. The eight hopping parameters in unit of eV for the six 1H-$MX_2$ monolayers and the calculated electronic polarization $\boldsymbol{P}$.

| | $MoS_2$ | $WS_2$ | $MoSe_2$ | $WSe_2$ | $MoTe_2$ | $WTe_2$ |
|---|---|---|---|---|---|---|
| $E_0$ | 1.751 | 1.893 | 1.683 | 1.767 | 1.516 | 1.603 |
| $t_{\rm E}$ | -0.353 | -0.382 | -0.382 | -0.412 | -0.456 | -0.499 |
| $t_{32}$ | -0.922 | -1.159 | -0.788 | -0.987 | -0.626 | -0.772 |
| $t_{23}$ | 0.122 | 0.210 | 0.065 | 0.139 | 0.022 | 0.099 |
| $t_{31}$ | -0.070 | -0.068 | 0.039 | 0.038 | -0.004 | -0.009 |
| $t_{13}$ | -0.008 | 0.088 | -0.037 | 0.031 | -0.093 | -0.041 |
| $t_{11}$ | 0.455 | 0.396 | 0.454 | 0.412 | -0.479 | 0.455 |
| $t_{22}$ | -0.182 | -0.189 | -0.150 | -0.161 | -0.095 | -0.103 |
| $\boldsymbol{P}$ | $(\frac{1}{3}, \frac{2}{3})$ | $(\frac{1}{3}, \frac{2}{3})$ | $(\frac{1}{3}, \frac{2}{3})$ | $(\frac{1}{3}, \frac{2}{3})$ | $(\frac{1}{3}, \frac{2}{3})$ | $(\frac{1}{3}, \frac{2}{3})$ |

there are $3 \times 3 \times 6 = 54$ nearest-neighbor hopping terms. The $D_{3h}$ symmetry provides that there are only eight independent terms including the crystal field effects [10], as listed in Eqs. (2) and (3) and Table S1. Next, we will show that both the band structure and topological property can be well captured by the multi-orbital model $H_s$ in Eq (1), while neglecting the $H'$. The amplitudes of $t_{31}$ and $t_{13}$ are small enough to be safely neglected. Though the finite hoppings $t_{11}$ and $t_{22}$ do have effects on the dispersion and the gap of the band structure, they have no contribution to nontrivial polarization due to their inversion-symmetric nature [12]. The nontrivial topological electronic polarization $\boldsymbol{P}$ comes from the inversion symmetry breaking, which can be well captured by the difference between $t_{23}$, $t_{32}$, and $t_{\rm E}$ included in $H_{\rm s}$. The effectiveness of the simplified model $H_{\rm s}$ is further verified via comparing the results of the eight-parameter model,

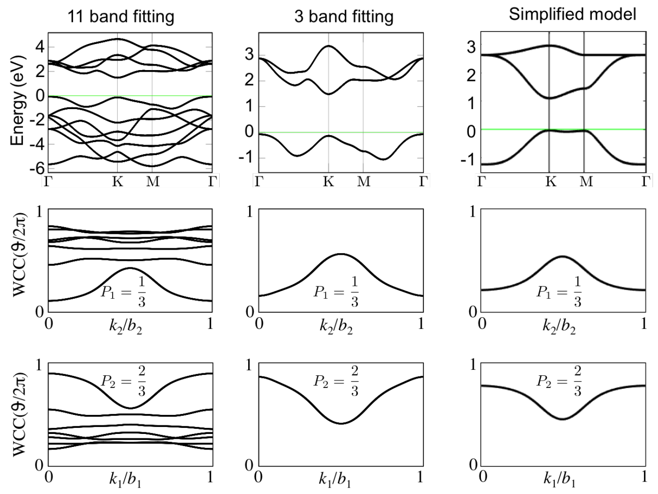


FIG. S3. Electronic bands and Wilson loops of a $MoS_2$ monolayer. The three columns are results from different tight-binding models. The results of 11 band fitting and 3 band fitting are from the WANNIER90 software. The parameters of the simplified model Eq. (1) are listed in Table I.

11-band fitting results from WANNIER90, and the first-principle calculations, as shown in Fig. S3.

In momentum space, the simplified Hamiltonian $H_{\rm s}(\boldsymbol{k})$ takes the matrix form as

$$H_{\rm s}(\boldsymbol{k}) = \begin{bmatrix} 0 & h_{12} & h_{13} \\ h_{12}^* & 0 & h_{23} \\ h_{13}^* & h_{23}^* & 0 \end{bmatrix}, \quad (4)$$

$$h_{12} = t_{\rm E} + t_{32} e^{ik_3} + t_{23} e^{-ik_3},$$

$$h_{13} = t_{\rm E} + t_{32} e^{-ik_2} + t_{23} e^{ik_2},$$

$$h_{23} = t_{\rm E} + t_{32} e^{ik_1} + t_{23} e^{-ik_1},$$

where $k_i = \boldsymbol{k} \cdot \boldsymbol{a}_i$ is defined in the 2D Brillouin zone.

### Supplemental C: Comparison to the multi-sublattice breathing kagome model

Here we compare our multi-orbital model with the breathing kagome model. As shown in Table I, the amplitude of $t_{23}$ is much smaller than that of $t_{32}$ and $t_E$ for the six 1H-$MX_2$ monolayers. When one neglect the effects from $t_{23}$, the above simplified multi-orbital model shares similarity to the multi-sublattice breathing kagome model, as shown in Fig. S4. In other words, the simplified model proposed for 1H-$MX_2$ here is a multi-orbital realization of the multi-sublattice breathing kagome model.

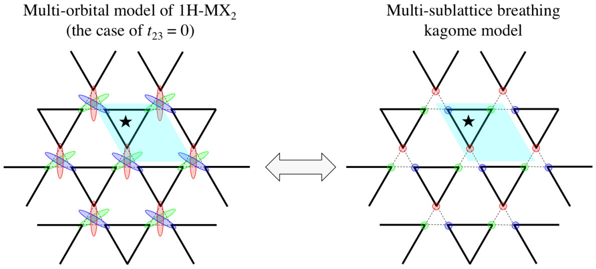


FIG. S4. Similarity between the simplified multi-orbital model of 1H-MX$_2$ to the multi-sublattice breathing kagome model. One rhombic unit cell is colored in cyan. The star marks the Wannier charge located at the hollow site in the unit cell, corresponding to an electronic polarization $\boldsymbol{P} = (\frac{1}{3}, \frac{2}{3})$.

## Supplemental D: More localized corner states in a passivated $MoS_2$ flake

There are dangling bonds and related edge states at an armchair edge of a $MoS_2$ flake. Figure 3 shows that the edge states (e.g. $n = 814$) are close to the in-gap corner states (e.g. $n = 808$) in energy, though a bulk $MoS_2$ monolayer has a relatively large band gap of about 2 eV. To reduce the interference from the dangling bond states, a passivated $MoS_2$ flake is constructed, as shown in Fig. S5(a). The Mo and S atoms at the outmost edge are passivated via bonding to oxygen (O) and hydrogen (H) atoms. The atom ratio of O and H atom is 1:2 to keep the $MoS_2$ flake charge neutral. Compared with the bare $MoS_2$ flake shown in Fig. 3, Fig. S5(a) shows that the corner states are farther away from other states in energy and more localized on the corners for a passivated $MoS_2$ flake.

The filling anomaly and corner states appear when there is nontrivial $\boldsymbol{P}$ for a TMD monolayer. The results of numerical simulations are presented in Fig. S5(b). The charge distribution of the corner states $n = 90$ in Fig. S5(b) matches well with the DFT results on the corner states $n = 1050$ in Fig. S5(a). It notes there is a difference in the state number $n$ because more orbitals are considered in the DFT calculations. In the lattice model simulation, we calculated the full charge distribution of the occupied bands. According to the definition of Eq. (6) in the Ref. [13], the filling anomaly is $\eta = 2$ for a $MoS_2$ monolayer that has $C_3$ symmetry. Thus 2 (4) of 3 (6) corner states are occupied for one spin (two spins) in a charge neutral flake. Taking the filling anomaly $\eta = 2$ into consideration when all the corner states are unoccupied, the system has four positive charges (2 for each spin). Calculating the full charge distribution of all the occupied states excluding the corner states while taking the ionic charge into consideration according to the definition $(\sum_{n=1}^{86} |\psi_n|^2 - 1)e$, we can see that there are $\frac{4|e|}{3}$ charges on each corner. It notes the $\frac{4|e|}{3}$ charge exactly comes from the lack of 4 corner states each of which has $-\frac{|e|}{3}$ charges on each corner.

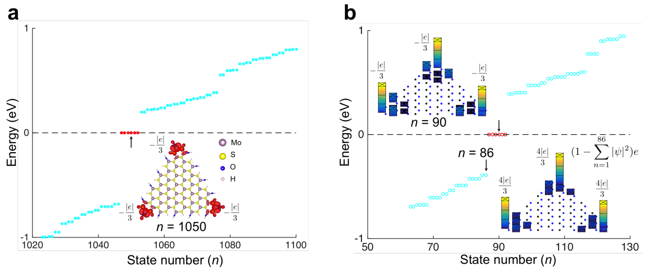


FIG. S5. Energy spectrum and corner states in a triangular flake within the size of 5 hexagons on each edge: (a) DFT results of a MoS2 flake, (b) simulations of the lattice model. The insets show the charge distributions of the corner states $n = 1050$ in (a) and $n = 90$ in (b). The inset in (b) also shows the full charge distribution of all the occupied states excluding the corner states while taking the ionic charge into consideration according to the definition $(\sum_{n=1}^{86} |\psi_n|^2 - 1)e$. There are $\frac{4|e|}{3}$ charges on each corner.

* Corresponding author: zengjiang@pku.edu.cn
† Corresponding author: xcxie@pku.edu.cn

[1] W. Kohn and L. J. Sham, Physical Review **140**, A1133 (1965).
[2] G. Kresse and J. Furthmüller, Computational Materials Science **6**, 15 (1996).
[3] G. Kresse and J. Furthmüller, Physical Review B **54**, 11169 (1996).
[4] P. E. Blöchl, Physical Review B **50**, 17953 (1994).
[5] J. P. Perdew, K. Burke, and M. Ernzerhof, Physical Review Letters **77**, 3865 (1996).
[6] D. C. Langreth and M. Mehl, Physical Review B **28**, 1809 (1983).
[7] A. D. Becke, Physical Review A **38**, 3098 (1988).
[8] H. J. Monkhorst and J. D. Pack, Physical review B **13**, 5188 (1976).
[9] A. A. Mostofi, J. R. Yates, Y.-S. Lee, I. Souza, D. Vanderbilt, and N. Marzari, Computer physics communications **178**, 685 (2008).
[10] G.-B. Liu, W.-Y. Shan, Y. Yao, W. Yao, and D. Xiao, Physical Review B **88**, 085433 (2013).
[11] J. Zeng, M. Lu, H. Liu, H. Jiang, and X. C. Xie, Science Bulletin **66**, 765 (2021).
[12] C. Fang, M. J. Gilbert, and B. A. Bernevig, Physical Review B **86**, 115112 (2012).
[13] W. A. Benalcazar, T. Li, and T. L. Hughes, Physical Review B **99**, 245151 (2019).
